# Supplementary material for: Electric selective activation of memristive interfaces in TaO$_x$-based devices
Source: arXiv:1908.03056 source file (2019-08-08)
Supplement: Supplementary file 1 [file SI.pdf]

**Supporting Information**

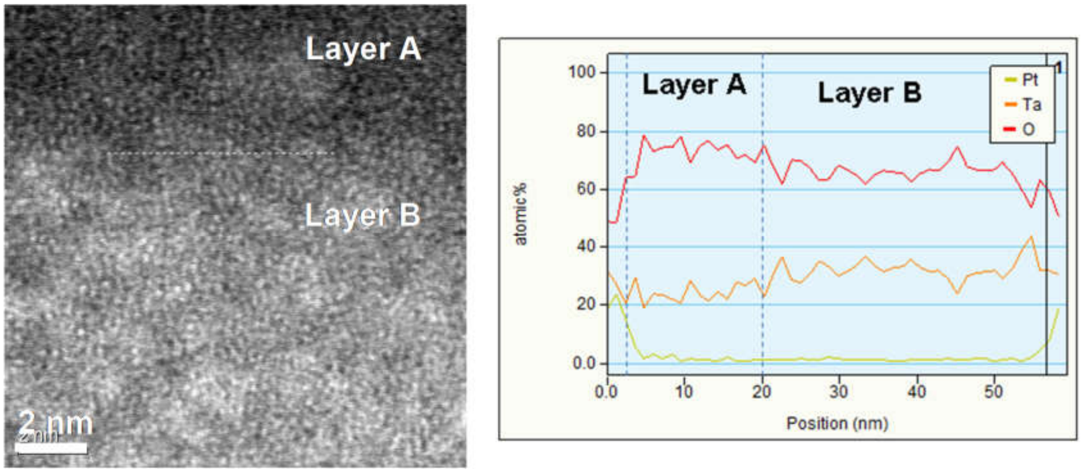


**Figure S1: (left) STEM-HAADF image taken at the interface between $TaO_x$ layers A (more oxidized, grown at 0.1mbar of $O_2$) and B (reduced, grown at 0.01mbar of $O_2$). Brighter zones correspond to Ta-rich clusters; (right) STEM-HAADF-EDX line scans, evidencing the difference in (average) Ta/O concentrations ratio between zones A ($Ta_2O_{4.7}$) and B ($TaO_{1.7}$).**

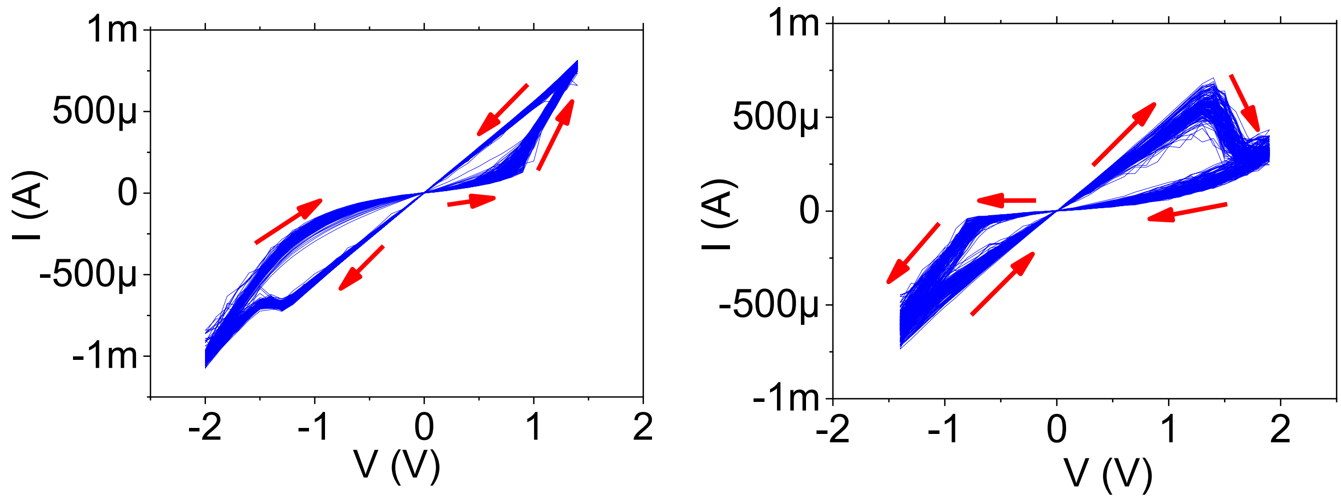


**Figure S2: Consecutive I-Vs, recorded for 200 cycles, with opposite circulations controlled by the voltage excursions $V_{max}$ and $V_{min}$. In both cases a rather stable and reproducible behavior is found.**

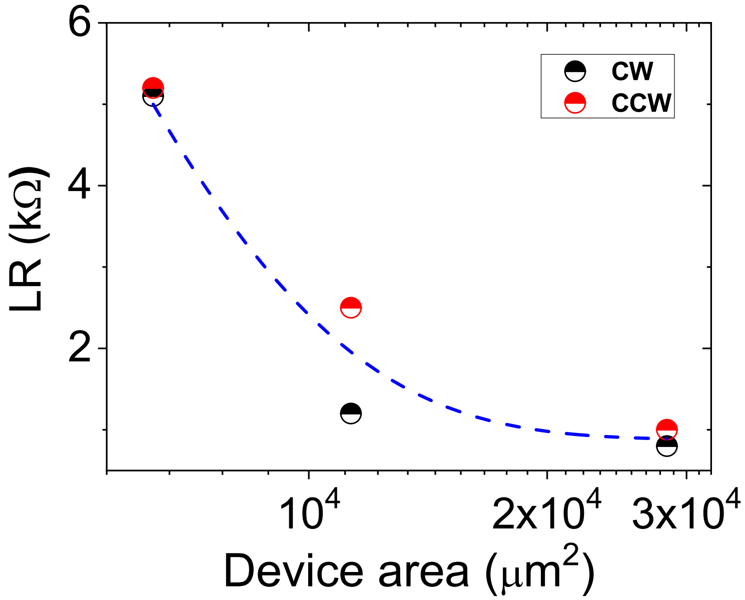


**Figure S3: Evolution of the LR state with the device area both for CW and CCW HSL's, indicating the presence of interface-related memristive behavior. The blue dashed line is a guide for the eye.**

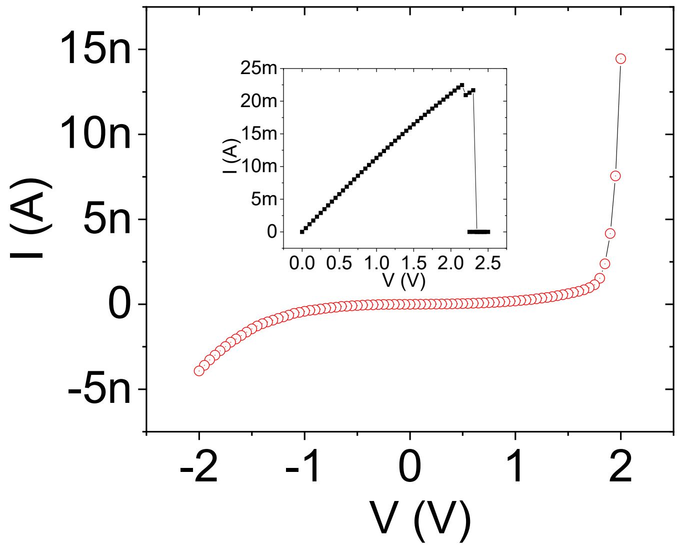


**Figure S4: Main panel: I-V curve obtained after forming pristine devices with positive stimuli, displaying a rectifying (Schottky) behavior. In this case, the insulating $Ta_2O_{5-x}$ layer is formed in contact with the top Pt electrode. Inset: electroforming process, displaying an abrupt resistance increase from a pristine low resistance state.**

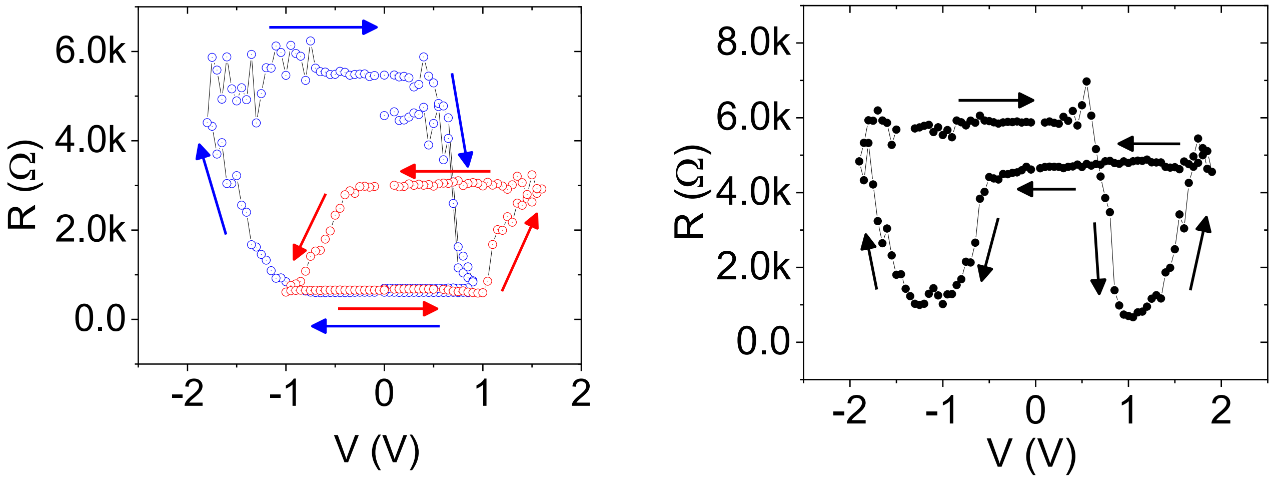


**Figure S5: Hysteresis switching loops displaying CCW and CW circulations (left, asymmetric stimuli) and "table with legs" (right, symmetric stimuli) for Au/$TaO_x$/Pt devices ($TaO_x$ is a bilayer similar to the one reported in the main text for Pt-Pt devices. The electroforming process was also similar in both cases). This evidences that the symmetry of the electric response follows the symmetry of the applied stimuli and is not determined by the device one.**

**Fitting procedure of current-voltage (I-V) curves in the $\gamma$ vs. $V^{1/2}$ representation**

The equivalent circuit model suggested by the $\gamma$ parameter analysis is the following:

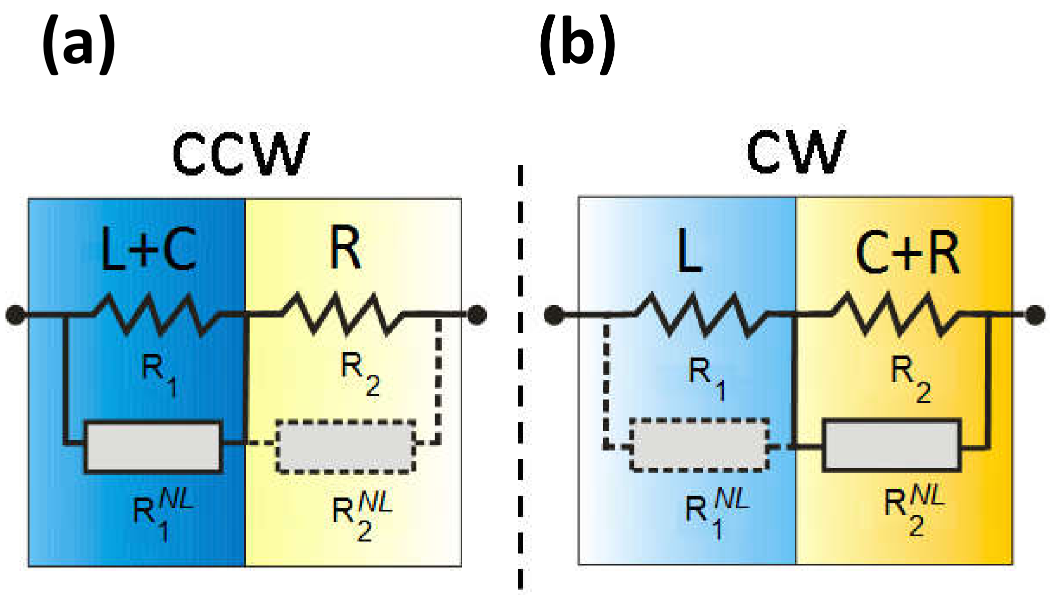


**Figure S6: Equivalent circuit model that describes (a) CCW HSL and (b) CW HSL. Ri indicate ohmic resistors, while $R_i^{NL}$ non-linear SCLC elements. L and R represent $Ta_{2-h}/Ta_2O_5$ and $Ta_2O_5/Ta_{2-y}$ interfaces, while C represents the bulk central $Ta_2O_5$ zone in between. The dashed-lines indicate that SCLC-non-linear element is short-circuited by the low resistance ohmic resistor in parallel.**

The corresponding I-V circuit-equations for the CCW HSL is given by

$$I = I_{R1} + I_{SCLC1} = (V - I_{R2}R_2)/R_1 + A_1(V - I_{R2}R_2)^{n_1}$$

where $I_{R1}$ and $I_{SCLC1}$ are the currents through $R_1$ resistor and the Space Charge Limited Conduction element $R_1^{NL}$, respectively. $A_1$ is a parameter related to the mobility, the dielectric constant and the width of Ta-oxide and $n_1$ is an exponent $\geq 2$.

This is an implicit equation that should be solved numerically in order to fit the experimental I-V by determining the fitting parameters $R_1$, $A_1$ and $n_1$. The short-circuited non-linear element $R_1^{NL}$ was discarded.

A similar procedure to fit the CW HSL case (only 1←→2 inversion is necessary) was followed.

## Parameters for numerical simulations with the VEOV model

In this section we determine the numerical values of the parameters employed in the VEOV simulations, in order to reproduce the experimental reported resistances values. According to Equation (2) of the main text, the resistivity of the 1D chain of domains for a given OV density profile is:

$$\rho = \rho_s - \rho_0\left[\sum_{i=1}^{N_L} A_L\delta_i - \sum_{i=N_L}^{N-N_R} A_C\delta_i - \sum_{i=N-N_R}^{N} A_R\delta_i\right], \quad \text{(s1)}$$

with $\rho_s = N\rho_0$, being $N$ the total number of sites and $\rho_0$ an effective resistivity to be determined. As we mentioned in the main text, the conversion from resistivity to resistance is a trivial scale factor that in the following we take equal to 1 for simplicity.

Taking into account that OV are mainly located at R zone for the $HR_1$ state and at L zone for the $HR_2$ state, we can approximate:

$$\rho_{HR_1} \approx \rho_s - \rho_0\left(A_R\delta_{0_T}\right), \quad \text{(s2)}$$

and

$$\rho_{HR_2} \approx \rho_s - \rho_0\left(A_L\delta_{0_T}\right), \quad \text{(s3)}$$

where $\delta_{0_T} = N\delta_0$.

The experimental values for the resistances are $HR_1 \approx 3.5$ kΩ and $HR_2 \approx 2$ kΩ, respectively. Therefore, assuming that $HR_1 - HR_2 = \rho_{HR1} - \rho_{HR2}$, we obtain:

$$\frac{1.5k\Omega}{\rho_0\delta_{0_T}} \approx (A_L - A_R) > 0 \therefore A_L > A_R. \quad \text{(s4)}$$

According to the model simulations, in the LR ($LR = LR_1 \approx LR_2$) state, OV are mainly located at the C zone of the active layer, thus:

$$\rho_{LR} \approx \rho_s - \rho_0 A_C\delta_{0_T}. \quad \text{(s5)}$$

Subtracting (s5) from (s2) and taking into account the experimental value for LR = 800 Ω we obtain:

$$A_C - A_R \approx \frac{2.7k\Omega}{\rho_0\delta_{0_T}}. \quad \text{(s6)}$$

Dividing (s6) by (s4) gives:

$$\frac{2.7k\Omega}{1.5k\Omega} \approx \frac{A_C - A_R}{A_L - A_R}. \quad \text{(s7)}$$

In our simulations we have chosen $A_C$=100 and $A_R$=10, consistently with the assumption that $A_C > A_L, A_R$. Thus, replacing these values in Equations. (s4), (s6) and (s7), we get:

$$(A_L - 10) \approx \frac{1.5k\Omega}{\rho_0\delta_{0_T}}, \quad \text{(s8)}$$

$$\frac{2.7k\Omega}{\rho_0 \delta_{0_T}} \approx 90 \quad \text{and} \tag{s9}$$

$$\frac{90}{A_L - 10} \approx \frac{2.7k\Omega}{1.5k\Omega} \ . \tag{s10}$$

A typical OV density value of $\delta_0 = 10^{20}cm^{-3}$ in $TaO_x$ thin films has been reported by Fleming *et. al*. (J. App. Phys. **88**, 850 (2000)).

In the VEOV model, we assign 100 sites to the active zone, which we assume roughly corresponds to 15 nm (the whole $Ta_2O_{5-x}$ layer is 15nm), giving 6.67 sites per nm. In a 1D approach, we consider that OV in a volumetric site collapse into a 1D nanodomain. Thus, we estimate $\delta_0 = 1x10^{-4}$ $sites^{-1}$ and $\delta_{0_T} = 100\delta_0$. Taking into account these values, we obtain after solving Equations (s8)- (s10), $A_L$=60 (satisfying $A_L > A_R$=10) and $\rho_0$ = 3 kΩ.

The other parameters employed in the VEOV simulation are the activation energies for OV diffusion, that we take $V_A = V_C = V_R \approx 0.1$ eV in units of the thermal energy.
